# Supplementary material for: Root-Growth of Boron Nitride Nanotubes: Experiments and \textit{Ab Initio} Simulations
Source: arXiv:1803.11374 ancillary file (2018-09-06)
Supplement: Supplementary file 1 [file supporting-information-root.pdf]

# Supporting Information of Root-Growth of Boron Nitride Nanotubes: Experiments and *Ab Initio* Simulations

Biswajit Santra[1],* Hsin-Yu Ko[1], Yao-Wen Yeh[2], Fausto Martelli[1], Igor Kaganovich[2], Yevgeny Raitses[2], and Roberto Car[1]†
[1]*Department of Chemistry, Princeton University, Princeton, NJ 08544, USA*
[2]*Princeton Plasma Physics Laboratory, Princeton, NJ 08543, USA*

## A1. EXPERIMENTAL SET-UP FOR ARC

Fig. S1 shows the current experimental set up in which the arc runs between two conductive electrodes made from tungsten. A separate boron target is immersed in the arc plasma, which serves as the boron feedstock for synthesis of boron nitride nanotubes (BNNTs). The boron target contains less than 0.1% impurities including metals. In previous studies,[1,2] electrodes were made with boron which simultaneously served as the boron feedstock. Since pure boron is a poor electrical conductor, in these prior experiments 2–4% metal impurities were added to the boron electrodes to make them electrically conductive, as needed for running the arc. The boron electrodes containing metallic impurities also served as the feedstock of boron for the synthesis of BNNTs.

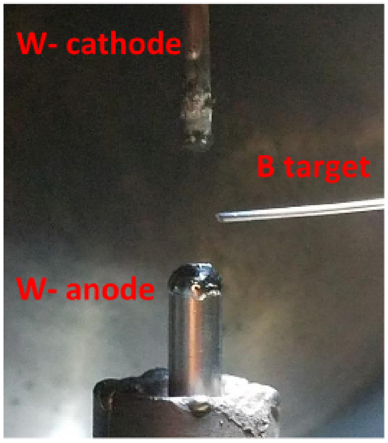


FIG. S1. A DC arc setup with two tungsten electrodes (cathode is top, anode is bottom) and the boron target for immersion to a nitrogen plasma produced by the arc. The target evaporated providing boron feedstock for synthesis of BN nanoparticles, including BNNTs.

## A2. EDS ANALYSIS

We have performed energy dispersive X-ray spectroscopy (EDS) on multiple tube-end nanoparticles to characterize their chemical contents. A typical EDS spectrum of the particles is shown in Fig. S2(b). The corresponding TEM image of the sample is also shown in Fig. S2(a). The EDS spectrum confirms that the tube-end nanoparticles are composed of boron, without transition metals. Also, as shown in Fig. S2(a), the boron nanoparticle is wrapped by two layers of boron nitride shell, which is the source of the nitrogen signal in the EDS spectrum. The additional features of silicon and copper appear from the background support material and are not attributed to the examined sample. Moreover, we find presence of oxygen which is thought to appear due to partial oxidations after the synthesis. The EDS spectrum clearly shows that tungsten or any other transition metals are absent in the tube-end nanoparticles, indicating

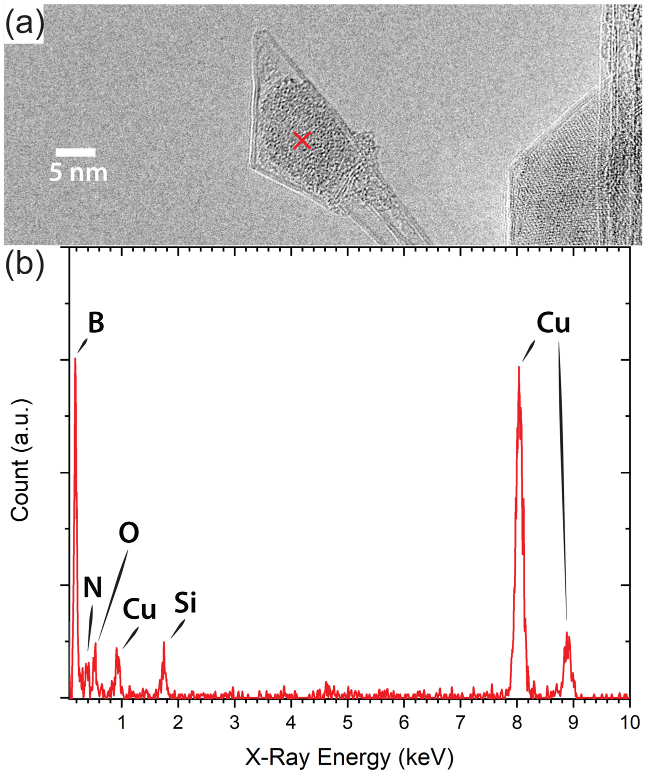


FIG. S2. (a) A TEM image of the BNNTs attached to a nanoparticle. The red cross indicates the position where EDS spectra were measured. (b) The EDS spectrum of the nanoparticle.

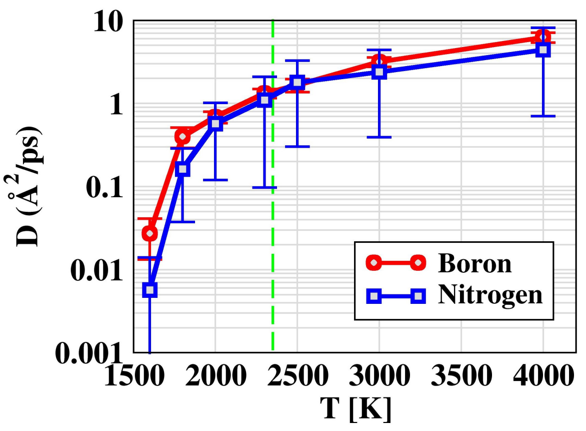


FIG. S3. The diffusivity (D) of boron and nitrogen atoms parallel to the surface computed from DFT-PBE simulations as a function of temperature. The green dashed line indicates the bulk melting temperature of boron.

that transition metals are not crucial for the synthesis of BNNTs using arc discharge.

## A3. DIFFUSIVITY OF BORON AND NITROGEN

We perform ab initio MD simulations of nitrogen in liquid boron at 1600–4000 K. In these simulations, the liquid slab contains 101 boron atoms and one nitrogen atom in the periodic unit. Each trajectory is at least 210 ps long. The diffusivity of boron and nitrogen atoms parallel to the surface is computed from the mean squared displacement (MSD) of the particles in a direction parallel to the surface of the slab. The entire trajectory was divided into sections of 20 ps each separated in time by 10 ps. In each section of the trajectory, the slope of the MSD is obtained from linear fitting and is set to be equal to 4D, as appropriate for two-dimensional diffusion. Then the average diffusivity and the standard deviation are computed from the values obtained from all sections of the trajectory. The temperature dependence of the diffusivity of boron and nitrogen is shown in Fig. S3. The statistical error is much larger for nitrogen than boron since the statistics are obtained from one nitrogen atom as opposed to 101 boron atoms.

## A4. TEMPERATURE DEPENDENCE OF BN STRUCTURES

We randomly place 12 nitrogen atoms on the surface of a liquid boron slab with periodic unit having surface area equal to 9.1×9.1 Å$^2$. Simulations at 3000 K produce a disordered BN mixture whereas at 2300 K they produce an ordered BN island, as shown in Fig. S4.

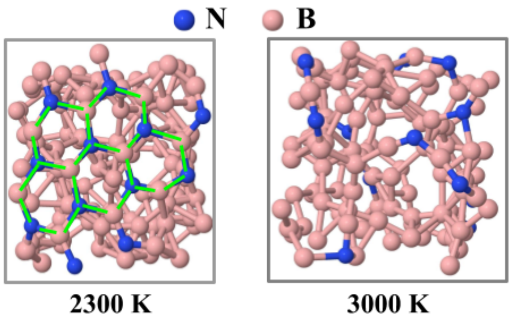


FIG. S4. Comparison of the BN structures at two different temperatures. The green lines highlight the hexagonal BN rings.

## A5. LOCAL ORDER PARAMETER ($S$)

In order to distinguish different BN structures we use a local order metric (LOM) that measures the degree of order in the neighborhood of an atomic site. The LOM maximizes the overlap between the spatial distribution of sites belonging to that neighborhood and the corresponding distribution in a suitable reference system.[3] The LOM takes a value close to zero for completely disordered environments and equal to one for environments that match perfectly with the reference. The site averaged LOM defines a scalar order parameter, $S$. To characterize the BN systems of interest here, we consider nitrogen sites only. The reference system is chosen to be the second coordination shell of a nitrogen atom in a perfect h-BN planar sheet, as shown in Fig. S5(a). This order parameter is able to distinguish different BN structures on the surface of liquid boron, as shown in Fig. S5.

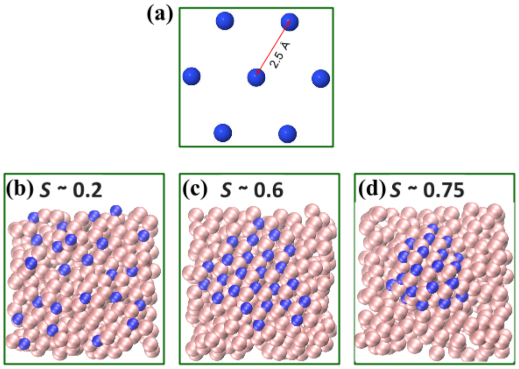


FIG. S5. (a) Reference system for the local order metric. The order parameter ($S$) in different structures: (b) randomly distributed nitrogen atoms on the boron surface, (c) a BN island on the surface, and (d) a BN cap on the surface. Each structure contains 25 nitrogen atoms.

## A6. STABILITY OF A BN CAP ON THE SURFACE OF LIQUID BORON

A (5,5) BN cap (containing 50 atoms) placed on a liquid boron surface (containing 100 atoms) floats on the surface and remains stable till the the entire time span of our simulation lasting more than 200 picoseconds at 2000 K, as shown in Fig. S6.

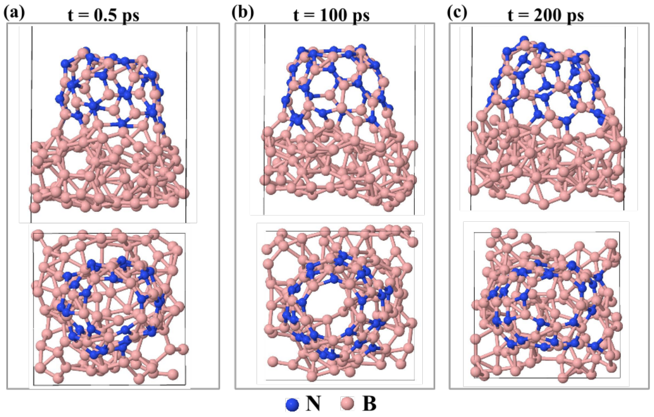


FIG. S6. Snapshots at different times (t) of a simulation in which a BN cap is placed on a liquid boron surface at 2000 K. Top and bottom panels are side and top views, respectively. See main article for further description.Snapshots at different times (t) of a simulation in which a BN cap is placed on a liquid boron surface at 2000 K. Top and bottom panels are side and top views, respectively. See main article for further description.

## A7. POSSIBLE ORIGIN OF THE NITROGEN ATOMS IN THE BORON DROPLETS

In the high-temperature synthesis of BNNTs, boron droplets form in the condensation of vapor containing boron and nitrogen atoms. Nitrogen atoms initially

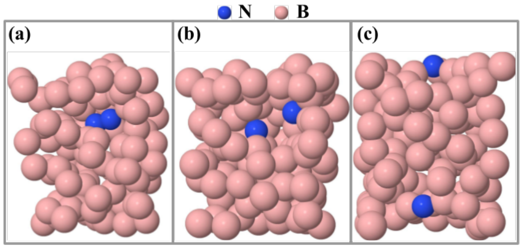


FIG. S7. Snapshots depicting the dissociation of an $N_2$ molecule initially located in a subsurface layer of a liquid boron slab at 2500 K. (a) Initial configuration showing an intact $N_2$ molecule. (b) Dissociation is already evident after 0.3 ps. (c) Both nitrogen atoms precipitate on the surface after ∼6.5 ps. A side view of the slab is shown in all the images.

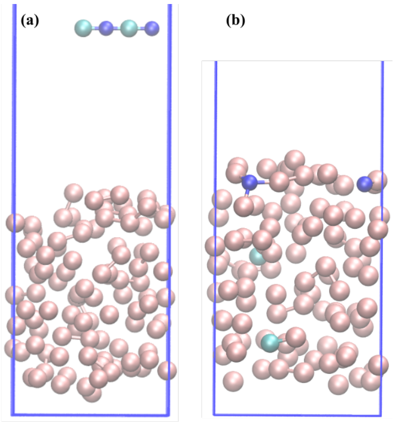


FIG. S8. Snapshots depicting the dissociation of a $(BN)_2$ chain that hits the surface of a liquid boron slab at 3000 K. (a) The $(BN)_2$ molecule moves towards the surface of the slab with thermal velocity. (b) The molecule dissociates within ∼0.5 ps as it hits the slab; the nitrogen atoms (blue) remain on the surface while the boron atoms (cyan) diffuse throughout the slab, shown in a side view.

present in the vapor may condense to form $N_2$ molecules or other molecular species, such as BN and BN chains. In order to confirm that such BN molecular species appear in arc, *in situ* spectroscopic measurements are required, which are beyond the scope of this work. In a study conducted previously during laser ablation of boron nitride in $N_2$ environment, the emission spectra showed signatures of BN in the ablated plasma plume.[4] This finding indicates that BN can also be present in arc plasma. These molecular species may get trapped into the boron droplets during their condensation, or they can get absorbed by droplets that are already formed. Inside the droplets all these nitrogen containing species dissociate quickly, as shown in Fig. S7 for $N_2$. BN chains hitting the surface of the droplet are easily adsorbed and dissociate quickly, as shown in Fig. S8 for a $(BN)_2$ molecule. A few trajectories similar to the one of Fig. S8 but involving an $N_2$ molecule indicate that this molecule is not easily adsorbed but tend to scatter off the droplet. This is a consequence of the weak interaction of $N_2$ with the boron surface. $N_2$ molecules would dissociate quickly if they could penetrate into the subsurface region (Fig. S7). Subsurface penetration of $N_2$ is a rare event on the time scale of our simulations and we are unable to quantify its likelihood by direct simulation.

## A8. BULK LIQUID BORON BENCHMARK

In order to assess the predictive power of our ab initio MD approach, we model bulk liquid boron and compare the simulated structure with x-ray diffraction experiments.[5] The simulation in the NVT ensemble uses a periodic simple cubic box containing 100 atoms. The lattice parameter is set equal to 11.5 Å to reproduce the

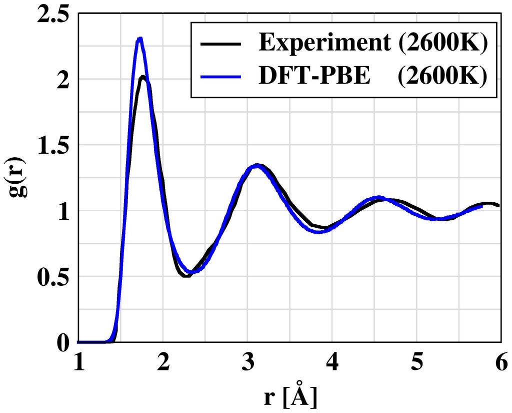


FIG. S9. A comparison of the radial distribution function, g(r), of liquid boron obtained from DFT-PBE simulation and from scattering experiment.

experimental density (2.3 g/cm$^3$) of liquid boron at the melting temperature (2350 K) and standard pressure using 200 boron atoms in the unit cell. The simulation runs for 50 ps following 10 ps of equilibration. The radial distribution function (RDF) at 2600 K agrees well with experiment at the same temperature, as shown in Fig. S9. The most notable difference between theory and experiment is a small discrepancy in the height of the first peak. This discrepancy may be due to the inaccuracy of the adopted DFT approximation but may also result from the experimental resolution (the highest momentum transfer was ~11 Å$^{-1}$). Notice that the RDF has not yet reached the asymptotic value of 1 at the boundary of our cell, suggesting that some size effects may affect our simulation.

* biswajit.santra@gmail.com
† rcar@princeton.edu

[1] J. Cumings and A. Zettl, Chem. Phys. Lett. **316**, 211 (2000).
[2] Y.-W. Yeh, Y. Raitses, B. E. Koel, and N. Yao, Sci. Rep. **7**, 3075 (2017).
[3] F. Martelli, H.-Y. Ko, E. C. Oğuz, and R. Car, Phys. Rev. B **97**, 064105 (2018).
[4] C. Dutouquet, S. Acquaviva, and J. Hermann, Spectrochimica Acta Part B: Atomic Spectroscopy **56**, 629 (2001).
[5] S. Krishnan, S. Ansell, J. J. Felten, K. J. Volin, and D. L. Price, Phys. Rev. Lett. **81**, 586 (1998).
